# Supplementary material for: Search for the decay $B^- \rightarrow \Lambda_c^+ \bar{p} \ell^- \bar{\nu}_{\ell}$ with the BABAR detector
Source: arXiv:1505.04733 source file (2015-05-18)
Supplement: Supplementary file 1 [file DataDrivenMLP.tex]

The comparison of \texttt{OnPeak} data and Monte Carlo, shown in Fig. \ref{fig:comp_TMVA_input_electron}, shows a deficit in the description of data by means of Monte Carlo simulations. To study the impact of this difference we perform a data driven training of the MLP, i.e. instead of Monte Carlo we use \texttt{OnPeak} data below $5.25 \gevcc$ as background sample.

For the electron channel the obtained ROC curve, i.e. background rejection efficiency vs. signal efficiency can be seen in Fig. \ref{fig:app:training_electron}, as well as the discriminator variable, given by the neural net. The comparison with Fig. \ref{fig:training_electron} shows that the ROC curve is nearly the same while the classifier distribution for background is flattened out for data in contrast to the Monte Carlo training where the background distribution shows a broad peak near $0$.
\begin{figure}[h]
  \subfigure[]{
    \includegraphics[width=.48\textwidth]{figures/TMVA/training/electron/DataDriven/ROC_curve}
    \label{subfig:app:ROC_electron}
  }
  \subfigure[]{
    \includegraphics[width=.48\textwidth]{figures/TMVA/training/electron/DataDriven/Classifier_dist}
    \label{subfig:app:Classifier}
  }
  \caption{ROC curve \subref{subfig:app:ROC_electron} and classifier distribution \subref{subfig:app:Classifier} for the MLP training for the electron channel.}
  \label{fig:app:training_electron}
\end{figure}

{\color{red} The sideband study might be helpful for systematic studies ...}
