# Supplementary material for: Search for the decay $B^- \rightarrow \Lambda_c^+ \bar{p} \ell^- \bar{\nu}_{\ell}$ with the BABAR detector
Source: arXiv:1505.04733 source file (2015-05-18)
Supplement: Supplementary file 2 [file DetermineCLFcut.tex]

\begin{figure}[h] \includegraphics[width=\textwidth]{figures/TMVA/cut/eChannel_bestCut_coarse}
  \caption{Comparison of stacked background Monte Carlo, scaled to data luminosity, and signal Monte Carlo for $\Bm \ra \LCp \antiproton \en \nueb$. Signal Monte Carlo is scaled to an {\it ad-hoc} branching fraction expectation of $1\times 10^{-4}$. The tested cut values range from $0.55$ to $0.95$ with a stepsize of $0.05$.}
  \label{app:fig:eChannel_bestCut_coarse}
\end{figure}
\begin{figure}[h]
\includegraphics[width=\textwidth]{figures/TMVA/cut/eChannel_bestCut_fine}
  \caption{Comparison of stacked background Monte Carlo, scaled to data luminosity, and signal Monte Carlo for $\Bm \ra \LCp \antiproton \en \nueb$. Signal Monte Carlo is scaled to an {\it ad-hoc} branching fraction expectation of $1\times 10^{-4}$. The tested cut values range from $0.91$ to $0.99$ with a stepsize of $0.01$.}
  \label{app:fig:eChannel_bestCut_fine}
\end{figure}
\begin{figure}[h] \includegraphics[width=\textwidth]{figures/TMVA/cut/muChannel_bestCut_coarse}
  \caption{Comparison of stacked background Monte Carlo, scaled to data luminosity, and signal Monte Carlo for $\Bm \ra \LCp \antiproton \mun \numb$. Signal Monte Carlo is scaled to an {\it ad-hoc} branching fraction expectation of $1\times 10^{-4}$. The tested cut values range from $0.55$ to $0.95$ with a stepsize of $0.05$.}
  \label{app:fig:muChannel_bestCut_coarse}
\end{figure}
\begin{figure}[h]
\includegraphics[width=\textwidth]{figures/TMVA/cut/muChannel_bestCut_fine}
  \caption{Comparison of stacked background Monte Carlo, scaled to data luminosity, and signal Monte Carlo for $\Bm \ra \LCp \antiproton \mun \numb$. Signal Monte Carlo is scaled to an {\it ad-hoc} branching fraction expectation of $1\times 10^{-4}$. The tested cut values range from $0.91$ to $0.99$ with a stepsize of $0.01$.}
  \label{app:fig:muChannel_bestCut_fine}
\end{figure}
