# Supplementary material for: Search for the decay $B^- \rightarrow \Lambda_c^+ \bar{p} \ell^- \bar{\nu}_{\ell}$ with the BABAR detector
Source: arXiv:1505.04733 source file (2015-05-18)
Supplement: Supplementary file 3 [file MLP_input.tex]

\begin{figure}[h]
  \subfigure[]{
    \includegraphics[width=.48\textwidth]{figures/TMVA/compare/electron/L2_stacked}
  }
  \subfigure[]{
    \includegraphics[width=.48\textwidth]{figures/TMVA/compare/electron/R2_stacked}
  }
  \subfigure[]{
    \includegraphics[width=.48\textwidth]{figures/TMVA/compare/electron/cosDthr_stacked}
  }
  \subfigure[]{
    \includegraphics[width=.48\textwidth]{figures/TMVA/compare/electron/cosBY_stacked}
  }
  \subfigure[]{
    \includegraphics[width=.48\textwidth]{figures/TMVA/compare/electron/YcandFitprob_stacked}
  }
  \subfigure[]{
    \includegraphics[width=.48\textwidth]{figures/TMVA/compare/electron/thetamiss_stacked}
  }
  \subfigure[]{
    \includegraphics[width=.48\textwidth]{figures/TMVA/compare/electron/pmiss_stacked}
  }
  \caption{Comparison of the different background sources with signal Monte Carlo for $\Bm \ra \LCp \antiproton \en \nueb$ for the input variables for the TMVA methods.}
  \label{fig:comp_TMVA_input_electron}
\end{figure}
\begin{figure}[h]
  \subfigure[]{
    \includegraphics[width=.48\textwidth]{figures/TMVA/compare/muon/L2_stacked}
   }
   \subfigure[]{
    \includegraphics[width=.48\textwidth]{figures/TMVA/compare/muon/R2_stacked}
   }
   \subfigure[]{
    \includegraphics[width=.48\textwidth]{figures/TMVA/compare/muon/cosDthr_stacked}
   }
   \subfigure[]{
    \includegraphics[width=.48\textwidth]{figures/TMVA/compare/muon/cosBY_stacked}
   }
   \subfigure[]{
    \includegraphics[width=.48\textwidth]{figures/TMVA/compare/muon/YcandFitprob_stacked}
   }
   \subfigure[]{
    \includegraphics[width=.48\textwidth]{figures/TMVA/compare/muon/thetamiss_stacked}
   }
   \subfigure[]{
    \includegraphics[width=.48\textwidth]{figures/TMVA/compare/muon/pmiss_stacked}
   }
  \caption{Comparison of the different background sources with signal Monte Carlo for $\Bm \ra \LCp \antiproton \mun \numb$ for the input variables for the TMVA methods.}
  \label{fig:comp_TMVA_input_muon}
\end{figure}
