# Supplementary material for: Search for the decay $B^- \rightarrow \Lambda_c^+ \bar{p} \ell^- \bar{\nu}_{\ell}$ with the BABAR detector
Source: arXiv:1505.04733 source file (2015-05-18)
Supplement: Supplementary file 4 [file fit_procedure.tex]

\begin{figure}[h]
  \includegraphics[width=\textwidth]{figures/TMVA/fit/clf_bkg_mu}
  \caption{$clf$ distributions, for $uds$, $c\bar{c}$, \BpBm and \BzBzb background Monte Carlo for the muon channel. None of the four background modes exhibits peaking background in the signal region at $+1$.}
  \label{fig:clf_bkg_zoom_mu}
\end{figure}
